# Supplementary material for: Image-Coupled Volume Propagation for Stereo Matching
Source: arXiv:2301.00695 source file (2022-12-30)
Supplement: Supplementary file 1 [file 06_appendix.tex]

\begin{figure*}[t]
\centering
\begin{subfigure}[t]{\dimexpr0.23\textwidth+12pt\relax}
    \makebox[15pt]{\raisebox{15pt}{\rotatebox[origin=c]{90}{\tiny{Image}}}}%
    \includegraphics[height=1in]
    {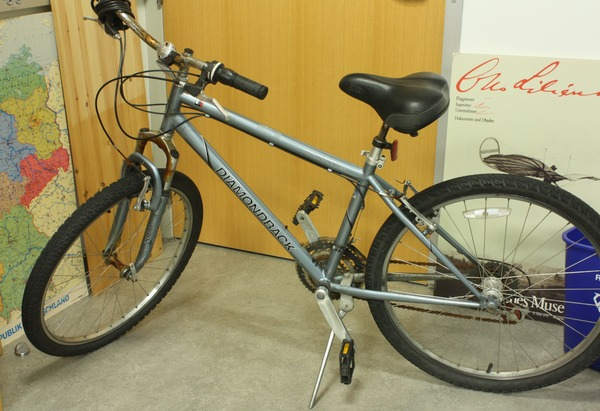}
    \makebox[15pt]{\raisebox{30pt}{\rotatebox[origin=c]{90}{\tiny{Blurred Ground Truth}}}}%
    \includegraphics[height=1in]
    {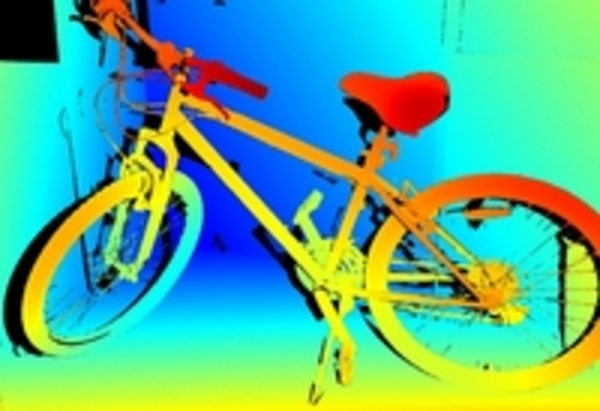}
    \makebox[15pt]{\raisebox{15pt}{\rotatebox[origin=c]{90}{\tiny{LEAStereo\cite{cheng2020hierarchical}}}}}%
    \includegraphics[height=1in]
    {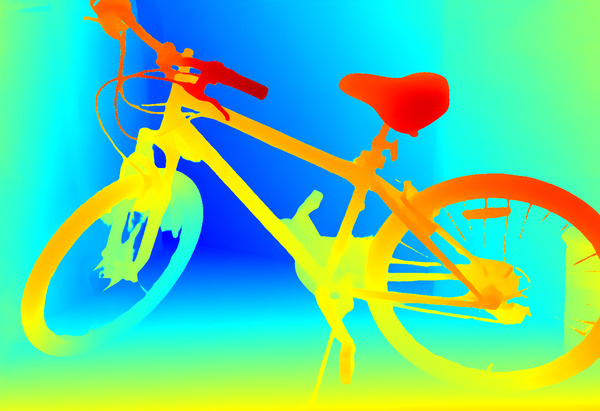}
    \makebox[15pt]{\raisebox{15pt}{\rotatebox[origin=c]{90}{\tiny{HITNet\cite{xu2022attention}}}}}%
    \includegraphics[height=1in]
    {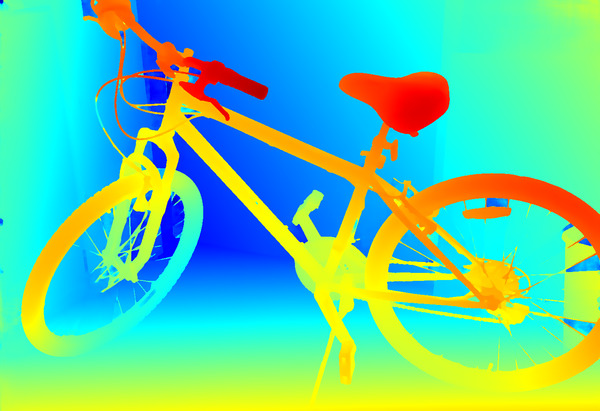}
    \makebox[15pt]{\raisebox{15pt}{\rotatebox[origin=c]{90}{\tiny{RAFT-stereo\cite{liu2022local}}}}}%
    \includegraphics[height=1in]
    {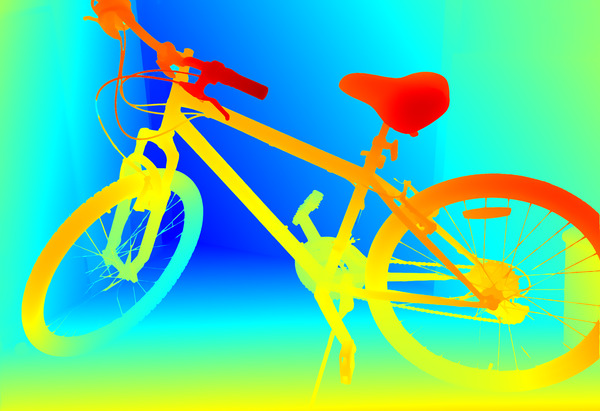}
    \makebox[15pt]{\raisebox{15pt}{\rotatebox[origin=c]{90}{\tiny{CREStereo\cite{shenpcw2022pcw}}}}}%
    \includegraphics[height=1in]
    {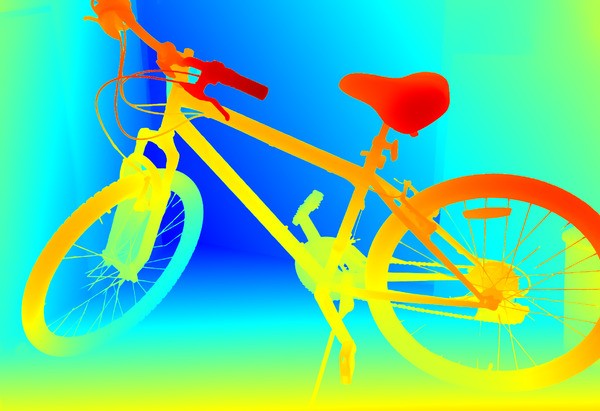}
    \makebox[15pt]{\raisebox{15pt}{\rotatebox[origin=c]{90}{\tiny{Ours}}}}%
    \includegraphics[height=1in]
    {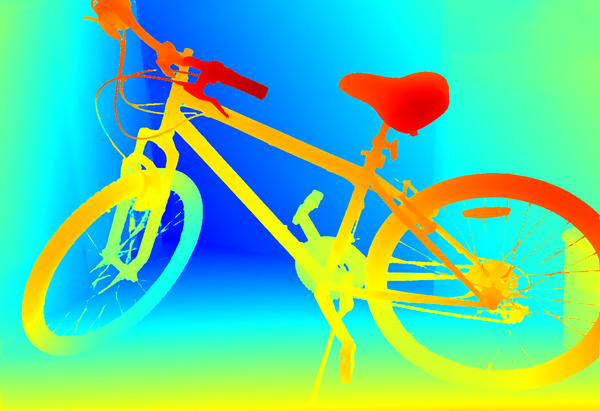}
\end{subfigure}
\begin{subfigure}[t]{0.23\textwidth}
    \includegraphics[height=1in]  
    {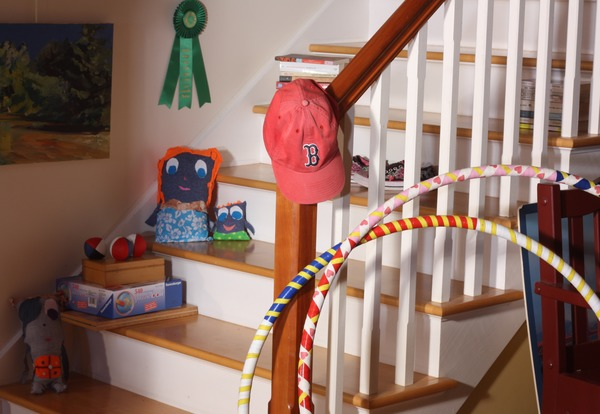}
    \includegraphics[height=1in]
    {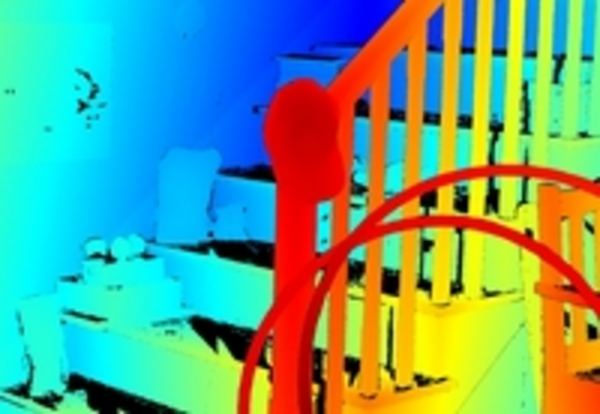}
    \includegraphics[height=1in]
    {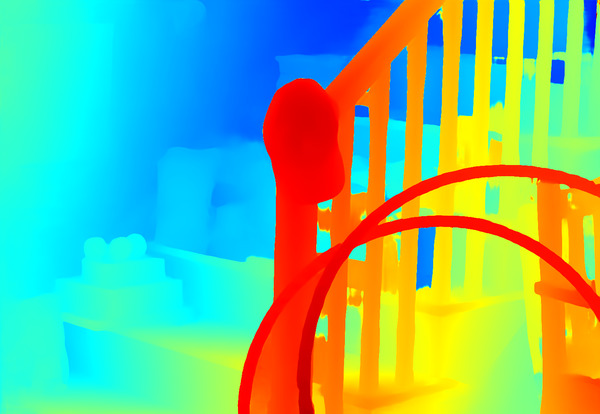}
    \includegraphics[height=1in]
    {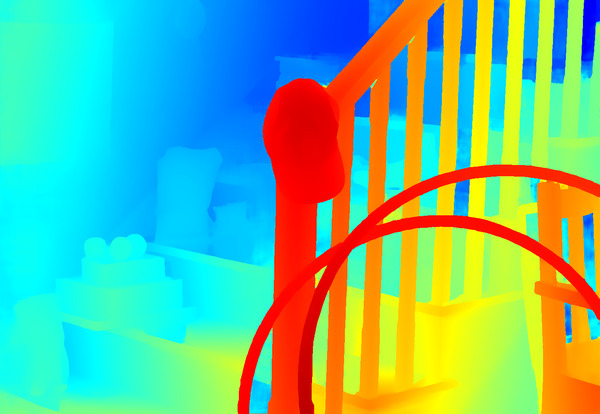}
    \includegraphics[height=1in]
    {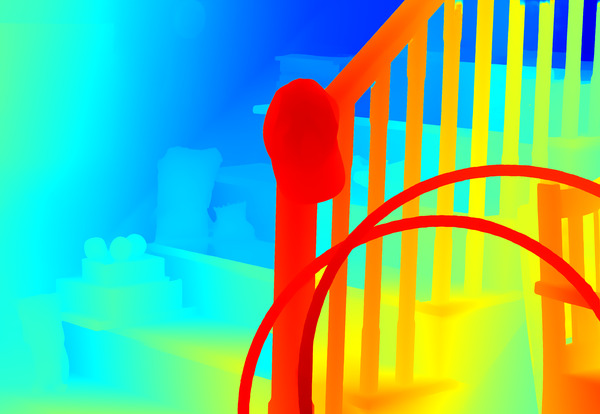}
    \includegraphics[height=1in]
    {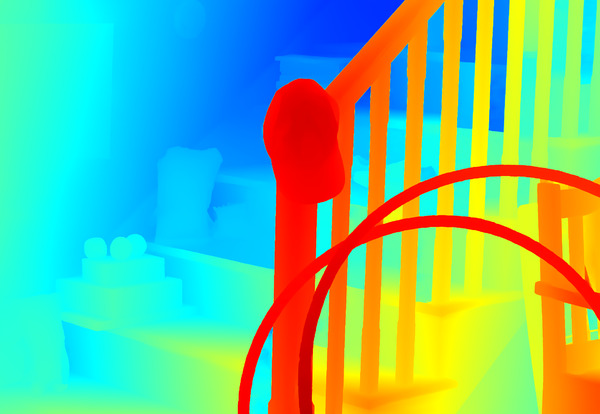}
    \includegraphics[height=1in]
    {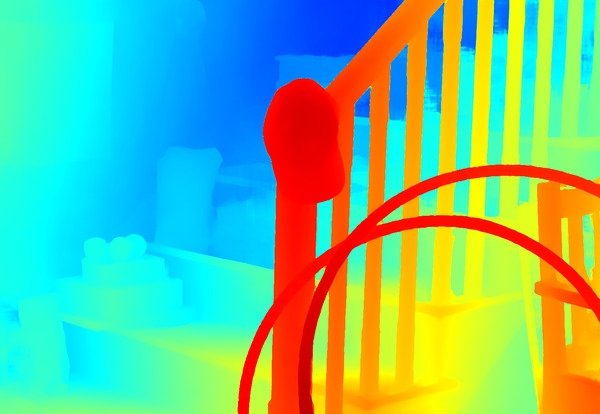}
\end{subfigure}
\begin{subfigure}[t]{0.23\textwidth}
    \includegraphics[height=1in]  
    {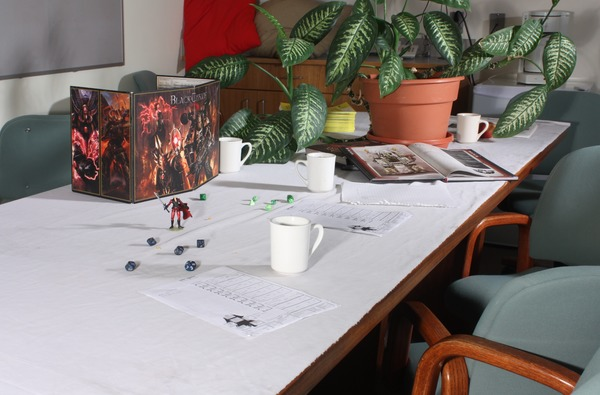}
    \includegraphics[height=1in]
    {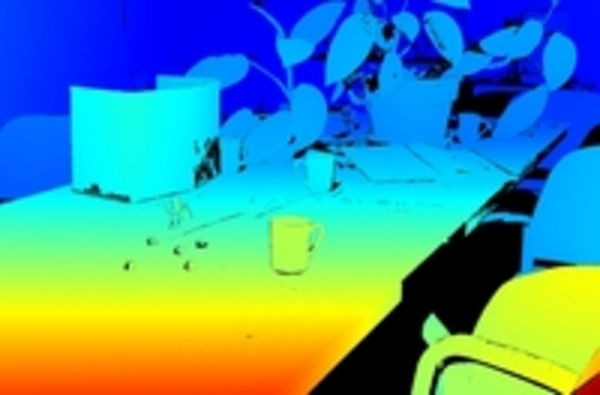}
    \includegraphics[height=1in]
    {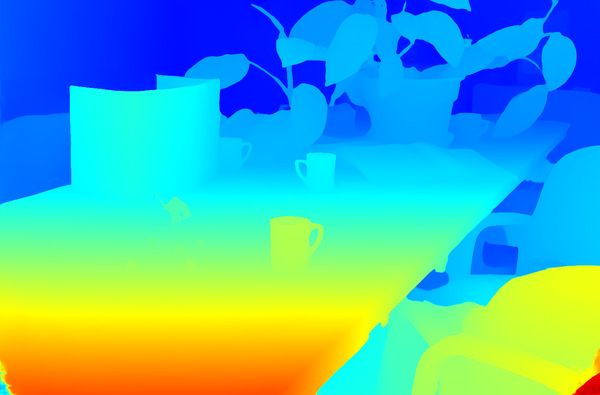}
    \includegraphics[height=1in]
    {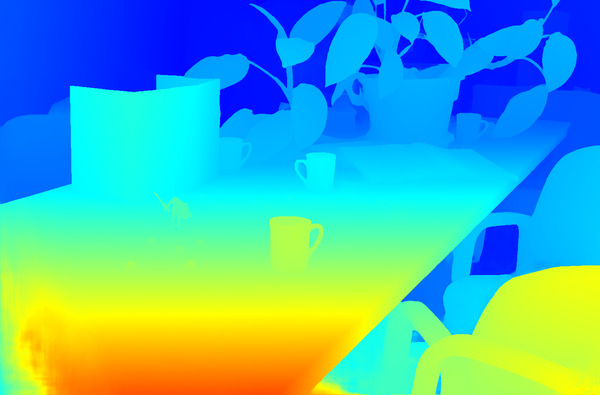}
    \includegraphics[height=1in]
    {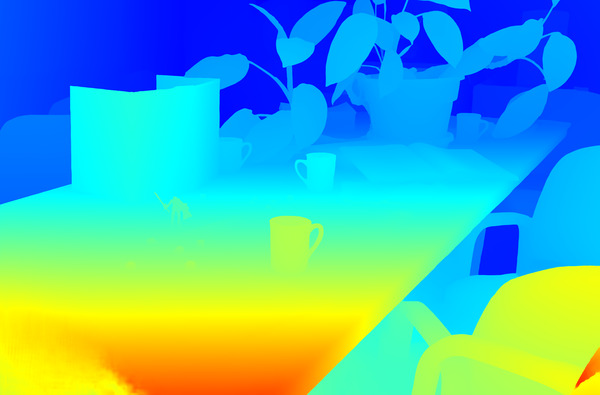}
    \includegraphics[height=1in]
    {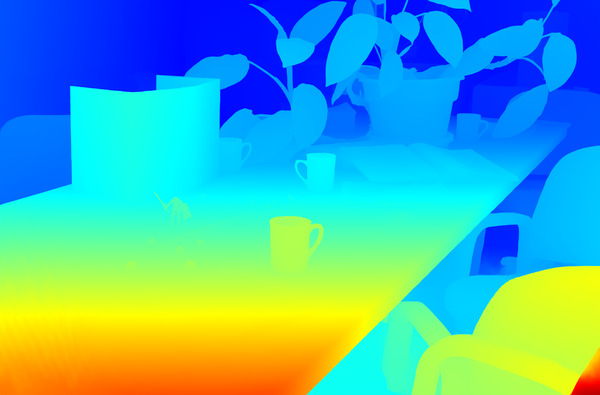}
    \includegraphics[height=1in]
    {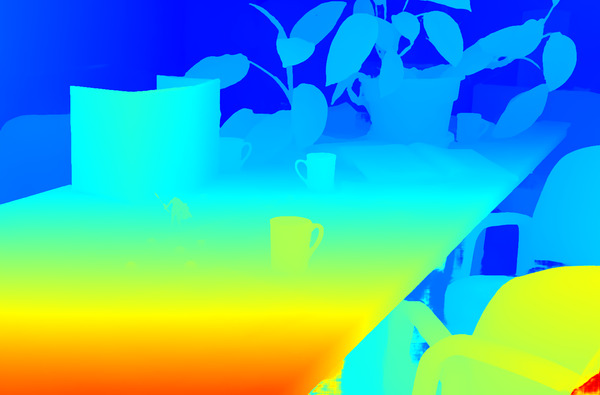}
\end{subfigure}
\begin{subfigure}[t]{0.23\textwidth}
    \includegraphics[height=1in]  
    {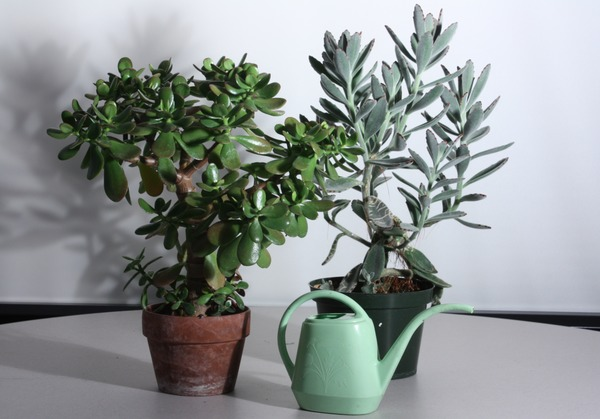}
    \includegraphics[height=1in]
    {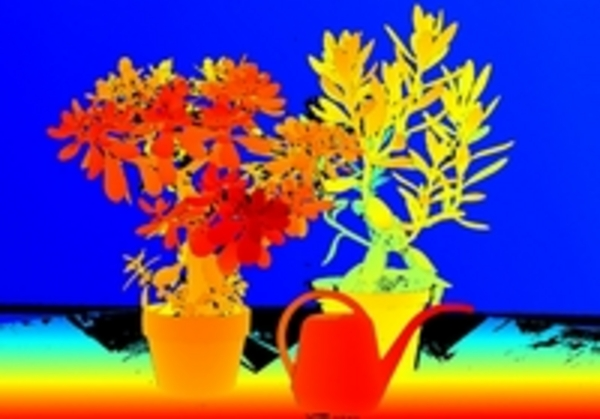}
    \includegraphics[height=1in]
    {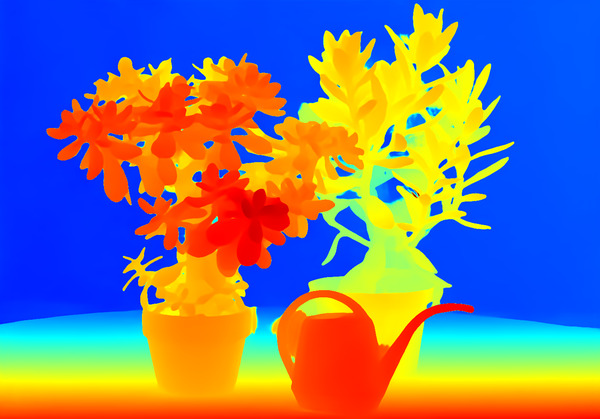}
    \includegraphics[height=1in]
    {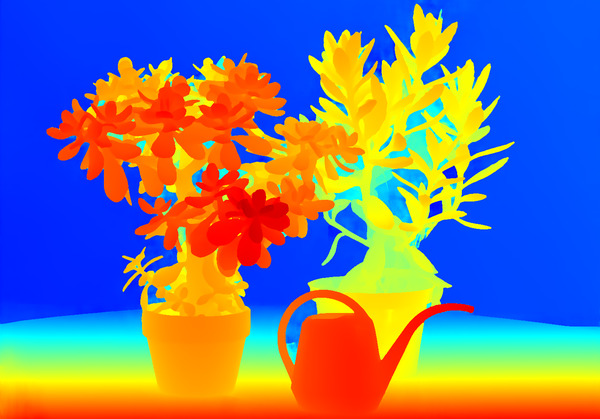}
    \includegraphics[height=1in]
    {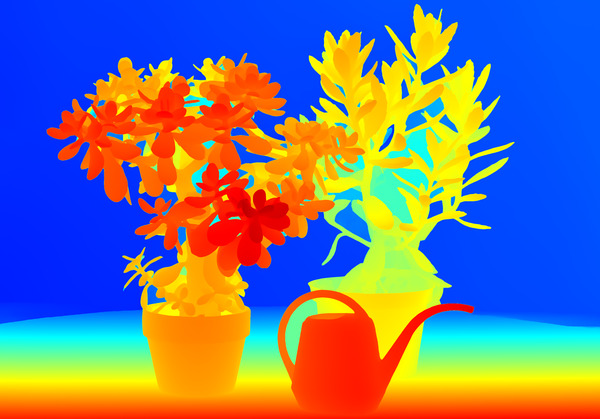}
    \includegraphics[height=1in]
    {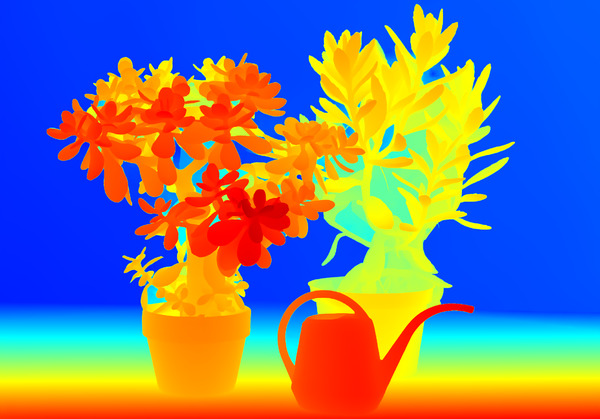}
    \includegraphics[height=1in]
    {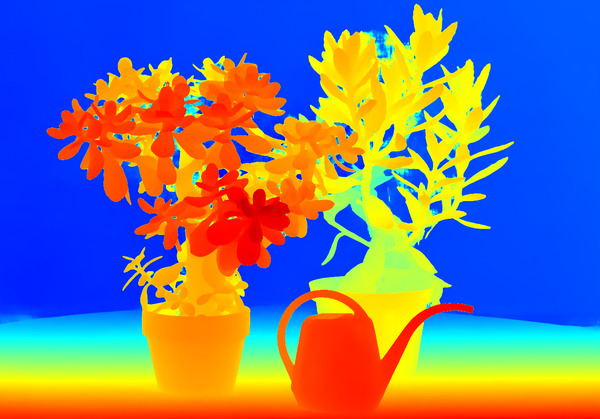}
\end{subfigure}

\caption{Qualitative Comparison on Middlebury V3}
\label{fig:mb_appendix}
\end{figure*}
